# Supplementary material for: AMED: Automatic Mixed-Precision Quantization for Edge Devices
Source: arXiv:2205.15437 source file (2024-06-10)
Supplement: Supplementary file 1 [file 060_appendix.tex]

%\appendix{}

% \crefalias{section}{appsec}
% \crefalias{subsection}{appsec}
% \crefalias{subsubsection}{appsec}

\section{Additional Experiments}
This appendix include the results for the Eyeriss hardware setup, as listed in Table \ref{tab:HW setup}.
The results are presented in Table \ref{tab:imagenet hw3} in this appendix and show that our method finds a different precision per layer for each model.
We also found that for a low memory boundary, our model chooses strategic layers to keep at high precision regardless of the size of the feature map, and tries to compensate for the latency over other layers.
More results and more experiments can be reproduced using the GitHub repository mentioned in this paper.

\begin{table*}[h!]
    \centering
    \begin{tabular}{@{}c c c c c c@{}}
    \hline
    Network & Method & Bitwidth & Acc (\%) & Latency (msec) & Size (MB) \\
    \hline
    \multirow{6}{7em}{ResNet-18} 
    & FP32 & 32/32 & 71.1 & ---  & 43.97\\
    & $LSQ_\psi$ & 8/8 & 70.0 & 3.42 & 14.68 \\
    & $LSQ_\psi$ & 4/4 & 68.73 & 0.85 & 7.34\\
    & HAWQv2 & $4_{MP}/4_{MP}$  & 70.22 & 2.94 & 8.52\\
    & MCKP & $3_{MP}/4_{MP}$  & 69.66 & 2.13 & 7.66\\
    & DDQ & $4_{MP}/4_{MP}$ & 71.2  & 2.22  & 7.83\\
    & \methodname{} & $2_{MP}/2_{MP}$  & 70.84  & \textbf{0.32} & 6.16 \\
    & \methodname{} & $2_{MP}/2_{MP}$  & 71.0 & \textbf{0.55} & 6.6\\
    \hline
    \multirow{8}{7em}{ResNet-50}
    & FP32 & 32/32 & 80.1 & --- & 102.06\\
    & $LSQ_{\psi}$ & 8/8 & 79.9 & 9.65 & 20.74 \\
    & $LSQ_{\psi}$ & 4/4 & 78.3 & 2.42 & 10.37 \\
    & $LSQ_\psi$ & 3/3 & 77.6 & 0.8 & 7.79\\
    & MCKP & $2_{MP}/4_{MP}$ & 75.28 & 3.22 & 7.96\\
    & HAWQv2 & $2_{MP}/4_{MP}$ & 76.1 & 7.82 & 10.13 \\
    % & BSQ & $2_{MP}/2_{MP}$ & 75.29 & new(101.4) & 10.82\\
    & \textbf{\methodname{}} & $2_{MP}/2_{MP}$ & \textbf{79.34} & \textbf{3.26} & 9.74\\
    & \textbf{\methodname{}} & $2_{MP}/2_{MP}$ & \textbf{79.43} & \textbf{3.45} & 9.75\\
    \hline
     \multirow{6}{7em}{MobileNetV2}
     & FP32 & 32/32 & 71.80 & --- & 17.86\\
     & $LSQ_{\psi}$ & 8/8 & 71.6 & 7.8 & 12.54\\
     & MCKP & $2_{MP}/8$ & 71.2 & 4.44 & 9.82\\
     & HAQ & $3_{MP}/3_{MP}$ & 70.9 & --- & --- \\
     & HAQ & $4_{MP}/4_{MP}$ & \textbf{71.47} & \textbf{2.03}  & 10.47\\
     & DDQ & $4_{MP}/4_{MP}$ & 71.8 & 5.87  & 10.217\\
     & PROFIT & $4_{MP}/4_{MP}$ & 71.5 & ---  & ---\\
     & LSQ + BR & $3/3$ & 67.4 & 3.9  & 11.429\\
     & \methodname{} & $2_{MP}/2_{MP}$ & {71.24} & \textbf{1.56} & 12.1\\
     & \methodname{} & $2_{MP}/2_{MP}$ & {70.97} & \textbf{1.21} & 9.53\\
    \hline
    \end{tabular}
    \caption{ The same comparison as in Table \ref{tab:imagenet} and the same notations, but with the latency from the simulator of the Eyeriss setup from Table \ref{tab:HW setup}. Note that our model yields a different bitwidth for each layer because the signal from the hardware is different in this setup. }
    \label{tab:imagenet hw3}
\end{table*}

\section{Bit Allocations}
\label{app:bit allocations}
In Fig. \ref{fig:res50 bits}, we add the bit allocation for ResNet-50 with a different hardware setup, and in Fig. \ref{fig:res18 bits}, we use different values for $\beta$ for ResNet-18.

One can see that both affect the bit allocation significantly towards building a more efficient network when the memory boundary is closer or when we increase the hardware constraints on the objective.

\begin{figure}
	\centering
% 	\vspace{-1.3cm}
	\includegraphics[width=1.\textwidth]{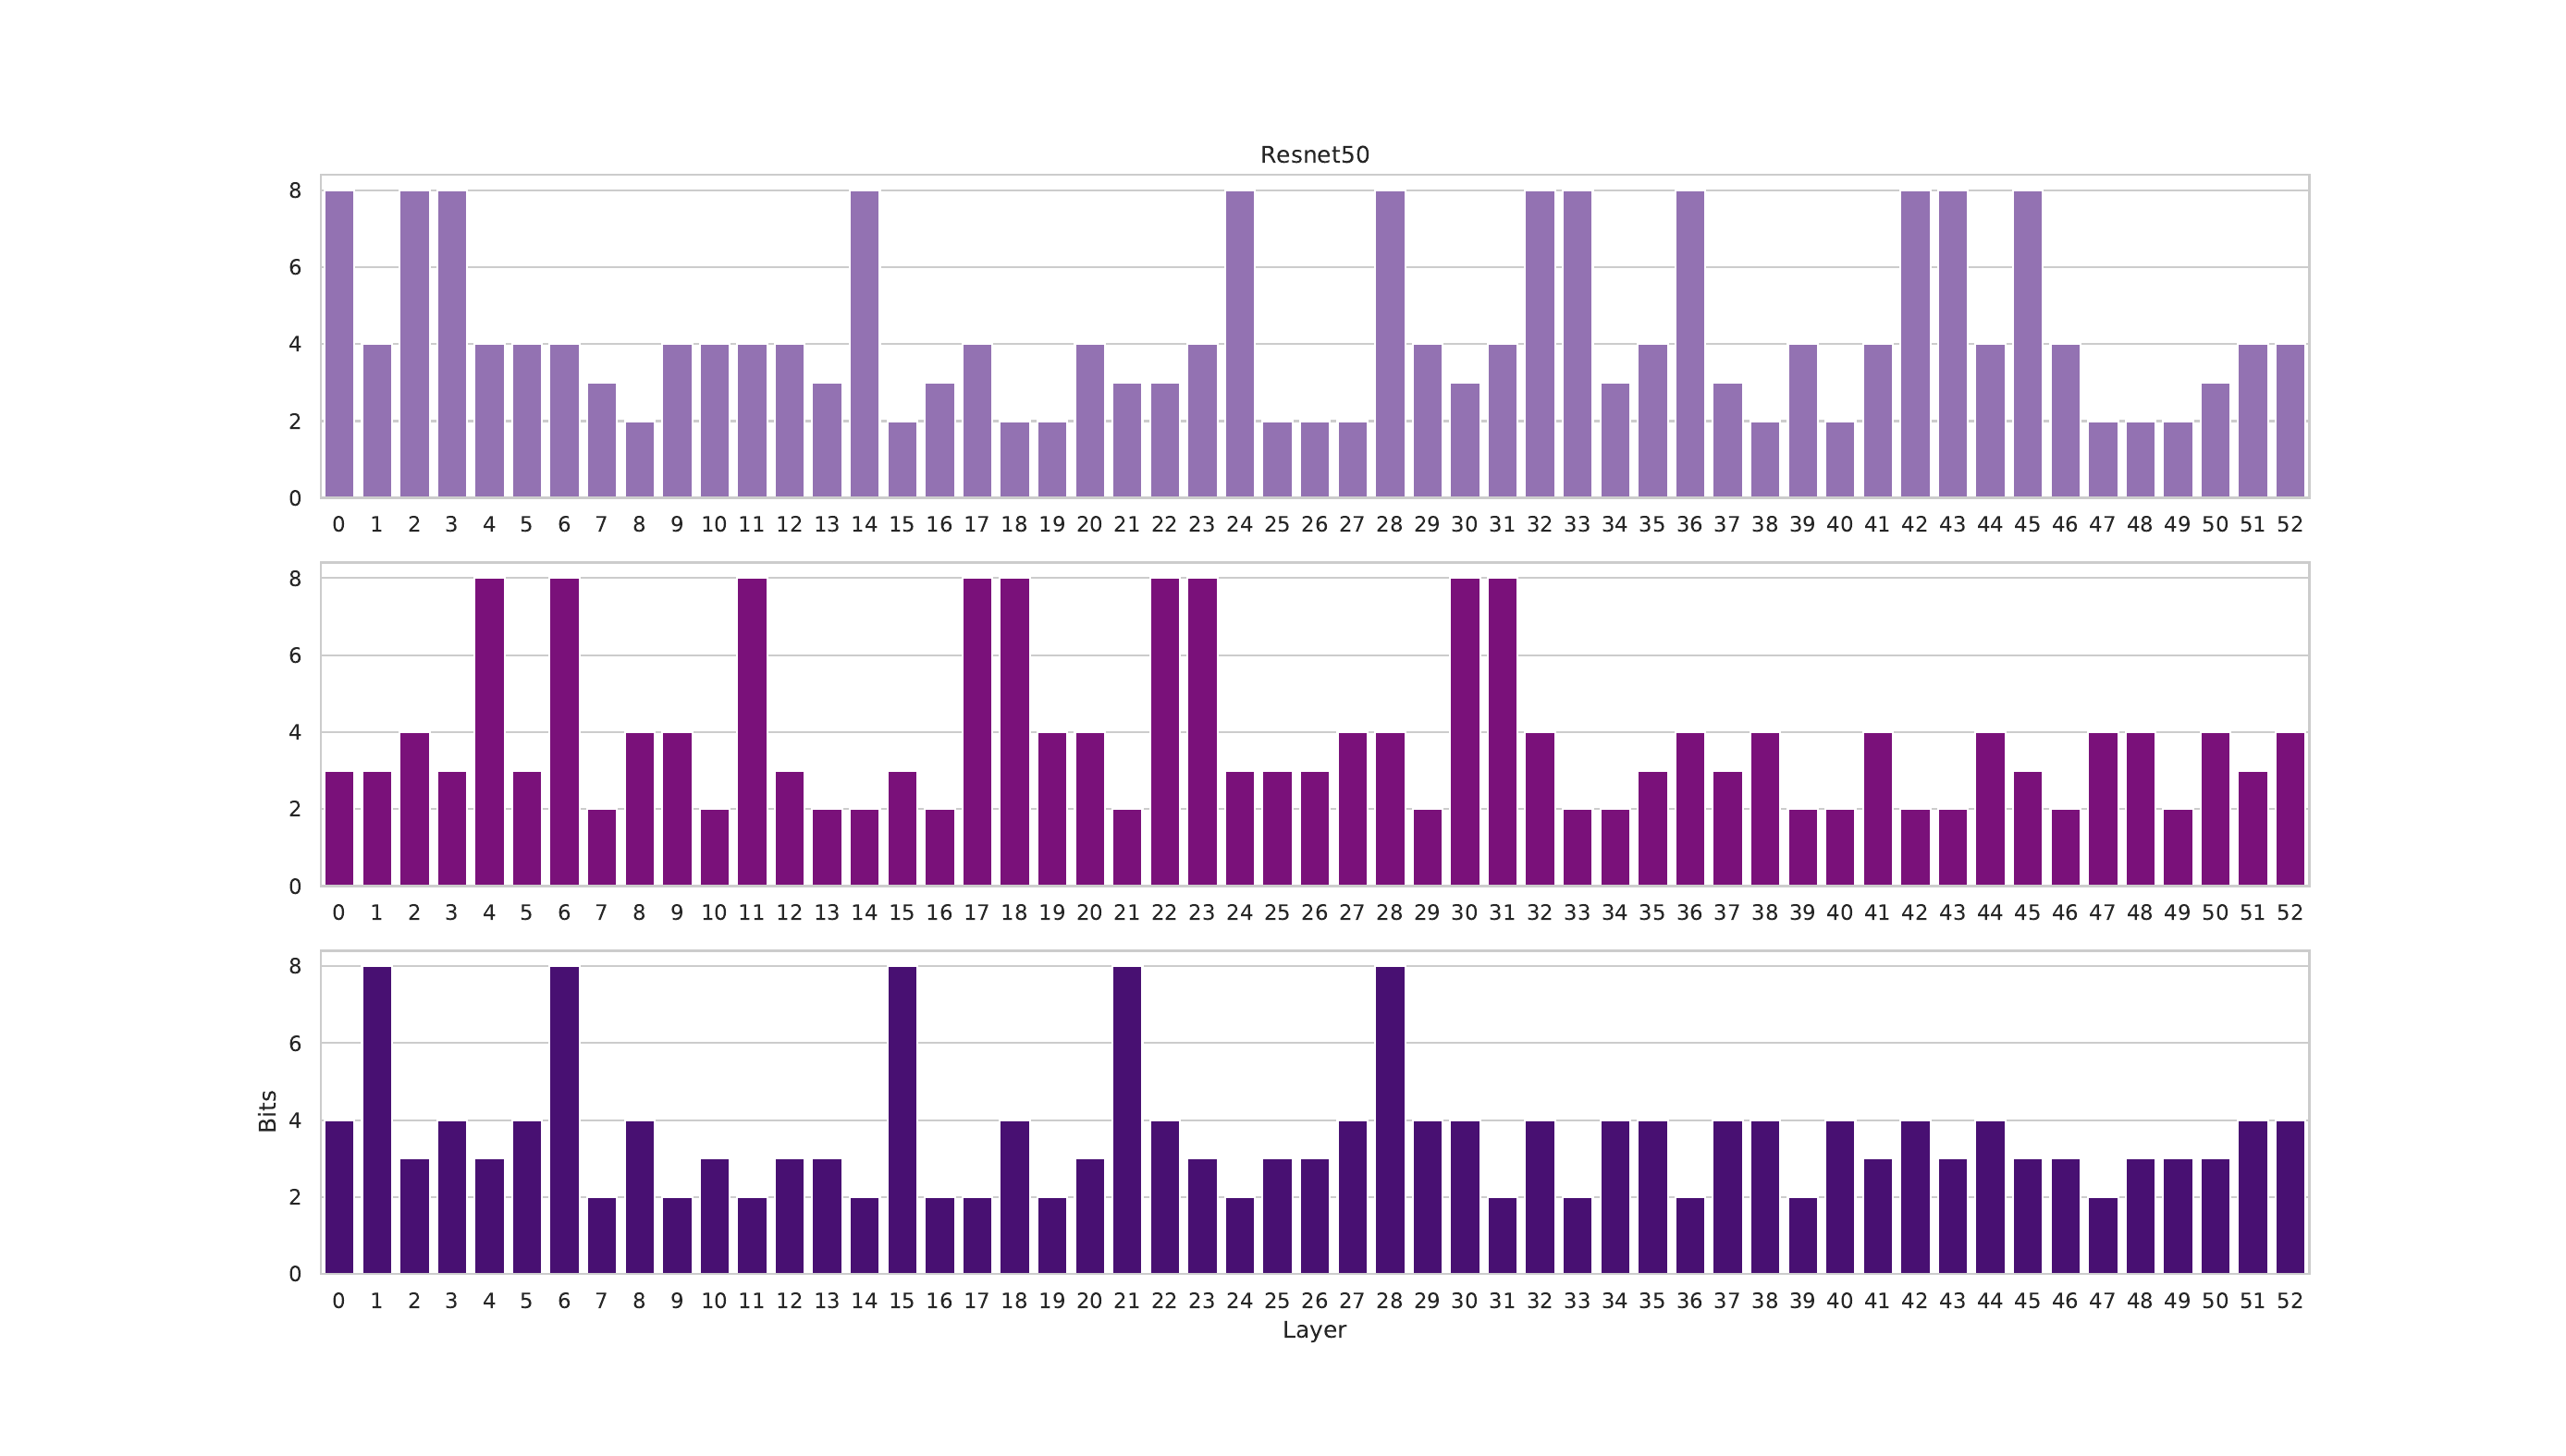} 
	\vspace{-0.3cm}
	\caption{Quantization bit allocation of ResNet-50 following our method using the simulator.
	The top figure is the SCALE-Sim setup, the middle is the Eyeriss setup, and the bottom is SCALE-Sim with low memory.}
	\label{fig:res50 bits}
\end{figure}

\begin{figure}[!ht]
\includegraphics[width=1.\textwidth]{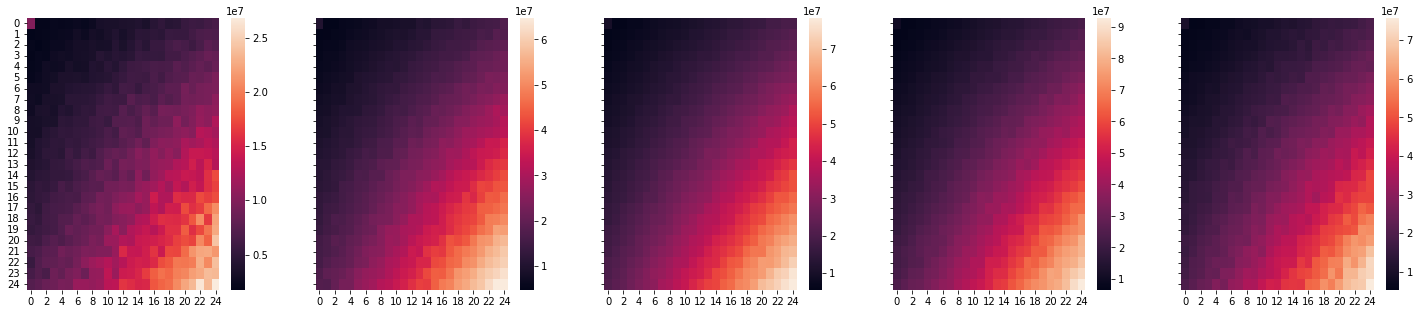} 
	\vspace{-0.3cm}
	\caption{Visualization of the loss surface of two subsequent layers of
ResNet18. At higher bit-width (left), the interactions between layers are
relatively small, making layer-wise optimization possible. On the other hand, at bit-width decrease (right), with
an increase of the quantization loss, the interactions become tangible and the loss is higher. A per layer optimization  depends on the initial point and potentially sub-optimal}
	\label{fig:LOSSES}
\end{figure}

\section{Reports}
\label{app:reports}
The simulator provides the following detailed reports about the performance during the inference of a CNN:
\begin{itemize}
    \item \textbf{Computation report}: Provides layer--wise details about Total Cycles, Stall Cycles, Overall Utilization, Mapping Efficiency, and Computation Utilization. An example is shown in Table \ref{tab:Compute report}.
    \item\textbf{Bandwidth report}: Provides layer--wise details about Average IFMAP SRAM Bandwidth, Average FILTER SRAM Bandwidth, Average OFMAP SRAM Bandwidth, Average IFMAP DRAM Bandwidth, Average FILTER DRAM Bandwidth, and Average OFMAP DRAM Bandwidth.
    \item \textbf{Detailed access report}: Provides layer--wise details about the number of reads and writes, and the start and stop cycles, for both of the above mentioned reports.
\end{itemize}

\begin{table*}[]
\centering
\begin{tabular}{llllll}
\textbf{LayerID} & Total   Cycles & Stall  & Overall Util \% & Mapping Efficiency \% & Compute Util \% \\
0& 137148& 0& 16.10753928     & 53.09483493& 16.10742183     \\
1& 132649& 0& 43.61369102     & 53.00234993& 43.61336223     \\
2& 36847& 0& 9.574727929     & 28.125& 9.574468085     \\
3& 61151& 0& 15.70538503     & 76.5625& 15.70512821     \\
4& 701907& 0& 71.27146118     & 76.38573961& 71.27135964     \\
5& 15483& 0& 24.68513854     & 40.625& 24.6835443      \\
6& 25283& 0& 21.22176957     & 76.04166667& 21.22093023     \\
7& 374807& 0& 71.87994421     & 75.31844429& 71.87975243     \\
8& 20187& 0& 28.399465       & 40.625& 28.39805825     \\
9& 25283& 0& 21.22176957     & 76.04166667& 21.22093023     \\
10& 374807& 0& 71.87994421     & 75.31844429& 71.87975243     \\
11& 5149& 0& 36.4002719      & 52.0625& 36.39320388     \\
12& 9399& 0& 25.28460475     & 74.265625& 25.28191489     \\
13& 157519& 0& 70.24724002     & 72.76722301& 70.24679406     \\
14& 6349& 0& 39.36052922     & 52.0625& 39.35433071     \\
15& 9399& 0& 25.28460475     & 74.265625& 25.28191489     \\
16& 157519& 0& 70.24724002     & 72.76722301& 70.24679406     \\
17& 6349& 0& 39.36052922     & 52.0625& 39.35433071     \\
18& 9399           & 0& 25.28460475     & 74.265625             & 25.28191489     \\
19& 157519& 0& 70.24724002     & 72.76722301& 70.24679406     \\
20& 3555& 0& 34.11392405     & 45.1171875& 34.10433071     \\
21& 6173& 0& 38.2998542      & 75.390625& 38.29365079     \\
22& 123129& 0& 76.17864191     & 77.54464286& 76.17802323     \\
23& 6243& 0& 38.8515137      & 45.1171875& 38.84529148     \\
24& 6173& 0& 38.2998542      & 75.390625& 38.29365079     \\
25& 123129& 0& 76.17864191     & 77.54464286& 76.17802323     \\
26& 6243& 0& 38.8515137      & 45.1171875& 38.84529148     \\
27& 6173& 0& 38.2998542      & 75.390625& 38.29365079     \\
28& 123129& 0& 76.17864191     & 77.54464286& 76.17802323     \\
29& 6243& 0& 38.8515137      & 45.1171875& 38.84529148     \\
30& 6173& 0& 38.2998542      & 75.390625& 38.29365079     \\
31& 123129& 0& 76.17864191     & 77.54464286& 76.17802323     \\
32& 6243& 0& 57.68861124     & 66.9921875& 57.6793722      \\
33& 11059& 0& 48.01858215     & 79.0234375& 48.01424051     \\
34& 262299& 0& 80.32093146     & 81.28125& 80.32062524     \\
35& 8931& 0& 60.48874706     & 66.9921875& 60.48197492     \\
36& 11059& 0& 48.01858215     & 79.0234375& 48.01424051     \\
37& 262299& 0& 80.32093146     & 81.28125& 80.32062524     \\
38& 8931& 0& 60.48874706     & 66.9921875& 60.48197492     \\
39& 11059& 0& 48.01858215     & 79.0234375& 48.01424051     \\
40& 262299& 0& 80.32093146     & 81.28125& 80.32062524     \\
41& 3827& 0& 58.33714398     & 64.59960938& 58.32190439     \\
42& 7103& 0& 51.84649092     & 71.92687988& 51.83919271     \\
43& 139231& 0& 72.87237576     & 73.39477539& 72.87185238     \\
44& 6131& 0& 60.69054803     & 64.59960938& 60.68065068     \\
45& 7103& 0& 51.84649092     & 71.92687988& 51.83919271     \\
46& 139231& 0& 72.87237576     & 73.39477539& 72.87185238     \\
47& 6131& 0& 60.69054803     & 64.59960938& 60.68065068     \\
48& 7103& 0& 51.84649092     & 71.92687988& 51.83919271     \\
49& 139231& 0& 72.87237576     & 73.39477539& 72.87185238     \\
50& 12263& 0& 60.31099649     & 64.20084635& 60.30607877     \\
51& 16043& 0& 61.18127844     & 73.03059896& 61.1774651      \\
52& 21471& 0& 2.916724885     & 3.057861328& 2.916589046    
\end{tabular}
    \caption{An example of the SCALE-Sim simulator computation report similar to \cite{MAX78000} for MobileNetV2 uniformly quantized to 2 bits (not including the FC-layer).
    }
    \label{tab:Compute report}
\end{table*}
